# Supplementary material for: A Graph-Based Approach for Category-Agnostic Pose Estimation
Source: arXiv:2311.17891 source file (2024-07-11)
Supplement: Supplementary file 1 [file 2_exp.tex]

\section{Methods Details}\label{supp:details}
\subsection{CaepFormer-T: An Enhanced Baseline}

We make two changes to CapeFormer architecture. First, we replace its Resnet-50~\cite{he2016deep} backbone with a comparable-sized stronger, transformer-based, SwinV2-T~\cite{liu2022swin} backbone. We also remove positional encoding because as found that it introduces an undesirable dependency on the order of the keypoints (further details in the main paper). Using these modifications we create an enhanced baseline called \textbf{CapeFormer-T}.

For completeness, we give a brief description of CapeFormer, whose design is similar to the DETR architecture and consists of 4 sub-networks:
\\
\begin{itemize}
\item \textbf{Shared backbone.} A pre-trained Resnet-50 is used to extract features from the input support and query images. 
To acquire the support keypoint features, we perform an element-wise multiplication between the support image feature map and keypoint masks. These masks are created by positioning Gaussian kernels centered at the support keypoints locations. In scenarios involving multiple support images, such as 5-shot settings, we calculate the average (in feature space) of the support keypoint features from different images.
This results in both the query feature map $\hat{F_q} \in \mathbb{R}^{hw \times C}$ and the support keypoint features $\hat{F_s} \in \mathbb{R}^{K \times C}$.
\item \textbf{Transformer encoder.} A transformer encoder is used to fuse information between the support keypoint features and the query patch features. The encoder consists of three transformer blocks, each housing a self-attention layer. Before entering the self-attention layer, the input support keypoints and query features are concatenated and subsequently separated once more. The outputs are refined query feature map $F_q$ and refined support keypoint features $F_s$.

\item \textbf{Similarity-Aware Proposal Generator.} The proposal generator aligns support keypoint features with query features, resulting in similarity maps. From these maps, we select peaks to serve as the similarity-aware proposals. In pursuit of a balance between efficiency and versatility, a trainable inner-product mechanism~\cite{shi2022represent} is employed to explicitly model similarity.

\item \textbf{Transformer decoder.} To decode keypoint locations from the query feature map, a transformer decoder network is utilized. The Transformer decoder consists of three layers, with each layer including self-attention, cross-attention, and feed-forward blocks.
An iterative refinement strategy, inspired by prior work~\cite{cai2018cascade, teed2020raft, zhu2020deformable}, is applied to enable each decoder layer to predict coordinate deltas for the previous coordinate predictions. 
Additionally, similar to the approach in Conditional DETR~\cite{meng2021conditional}, the decoder utilizes the predicted coordinates to provide enhanced reference points for pooling features from the image feature map.
\\
\end{itemize}

\subsection{Alternative Designs}
\subsubsection{Graph Prior As Loss Functions}
A na\"ive approach to utilizing the graph structure is to force features of the support and query image to be similar along an edge, which is defined by a straight line between 2 keypoints. Denote the feature map of support and query images as $F_s$ and $F_q$ respectively. Given an edge $e \in E$, we sample the feature maps $k$ times along the edge from both feature maps to acquire $\{f_s^{e,i}, f_q^{e,i}\}, i \in [1, k]$. We then encourage the cosine similarity between $f_s^{e,i}$ and $f_q^{e,i}$ to be large:

\begin{equation}
L_{skeleton} = \sum_{e \in E} \sum_{i=1}^k (1-\frac{f_s^{e,i} \cdot f_q^{e,i}}{\lVert f_s^{e,i} \rVert \lVert f_q^{e,i} \rVert})
\end{equation}

This solution didn't improve performance. First, we had the strong assumption that the features along a straight line should be similar, which doesn't always hold. Second, this loss resulted in a smoother heatmap, as we only required the similarity of sampled features, while we should encourage distinct features to localize the keypoints.

Thus, we forced the cosine similarity between $f_s^i$ and $f_q^j$ to be large for $i=j$ and small for $i \neq j$. However, this constraint was too restrictive and resulted in worse performance.

% Look twice
\subsubsection{Alternative Architecture Choices}
We asses a look-forward twice scheme~\cite{zhang2022dino, jia2023detrs}, which is common in DETR architectures, to leverage the refined coordinates information derived from previous decoder layers. Although shown effective in detection tasks, we observed it did not improve performance for our keypoint localization task.

\section{Further Experiments}\label{supp_exp}
\label{sec:exp}
\subsection{Model Scalability}

\subsubsection{Backbone Size.}
We show that our design scales better than previous methods. Similar to DETR-based models, employing a larger backbone improves performance. 
We employ a stronger backbone, SwinV2-S, on both CapeFormer and our graph-based design. Results in Table~\ref{Tab:supp_mp100}.
As shown, our graph design also enhances the performance for larger backbones, improving results by 0.83\% under 1-shot setting over CaprFormer-S.

\begin{table*}
\centering
\caption{
\textbf{Larger Backbone MP-100 Results.} PCK performance under 1-shot settings using a larger backbone. Our approach consistently outperforms other methods, and specifically CapeFormer-S, which uses the same backbone, across all splits.}
\begin{tabular}{cc c|ccccc | c}

\toprule
&& \textbf{Model} & Split 1 & Split 2 & Split 3 & Split 4 & Split 5 & Avg \\
% & \multicolumn{6}{c}{1-Shot} \\
\midrule
\multirow{7}{*}{\textbf{1-Shot}} && ProtoNet~\cite{snell2017prototypical} & 46.05 & 40.84 & 49.13 & 43.34 & 44.54 & 44.78 \\
&& MAML~\cite{finn2017model} & 68.14 & 54.72 & 64.19 & 63.24 & 57.20 & 61.50 \\
&& Fine-tuned~\cite{nakamura2019revisiting} & 70.60 & 57.04 & 66.06 & 65.00 & 59.20 & 63.58 \\
&& POMNet~\cite{xu2022pose} & 84.23 & 78.25 & 78.17 & 78.68 & 79.17 & 79.70 \\
&& CapeFormer~\cite{Shi_2023_CVPR} &  89.45 & 84.88 & 83.59 & 83.53 & 85.09 & 85.31 \\
\cmidrule(lr){2-9}

&& CapeFormer-S &  93.36  & 89.28 & 89.68 & 87.37 & 89.57 & 89.85 \\
&& \textbf{GraphCape-S} & \textbf{94.73} & \textbf{89.79} & \textbf{90.69} & \textbf{88.09} & \textbf{90.11} & \textbf{90.68} \\

\bottomrule
\end{tabular}
\label{Tab:supp_mp100}
\end{table*}

\subsubsection{Number of Decoder Layers.} We evaluate the impact of incorporating additional decoder layers into our architecture. Results are shown in Figure~\ref{fig:decoder_layers}. As can be seen, employing a larger number of decoder layers using our graph design shows better scalability, with boosted performance compared to CapeFormer-T for any number of decoder layers tested. We chose to use only 3 decoder layers in our quantitative and qualitative comparisons for a fair comparison with the original CapeFormer.

\begin{figure}
	\centering
	\includegraphics[width=0.9\textwidth]{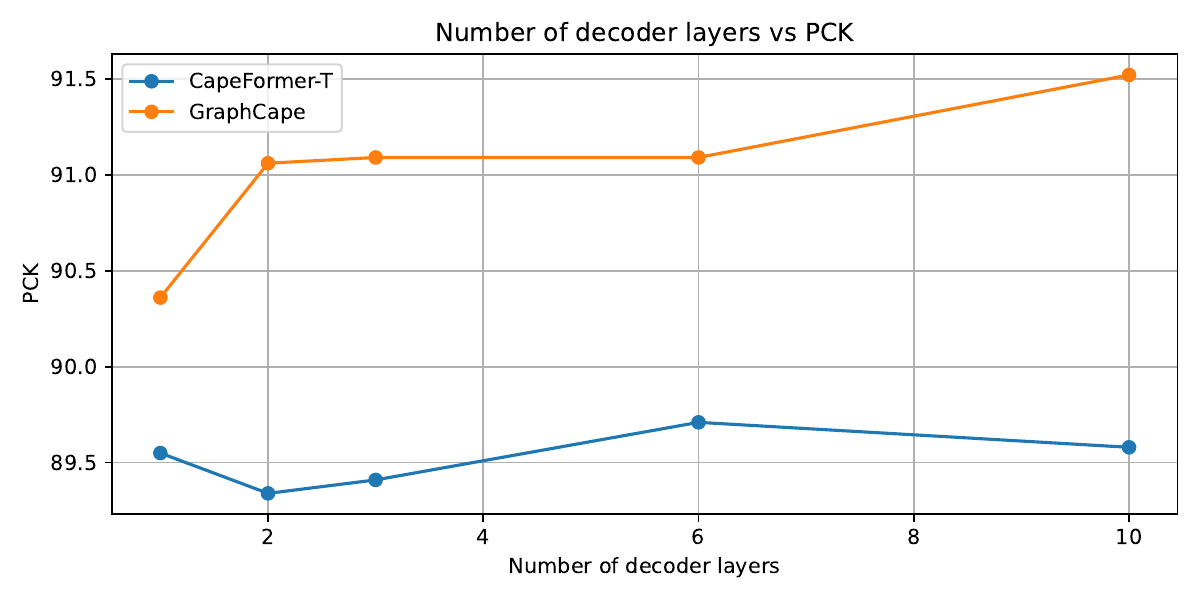}
	\caption{\textbf{Number of Decoder Layers.} Utilizing a higher number of decoder layers through our graph-based model demonstrates improved scalability, consistently enhancing performance compared to CapeFormer-T across various tested numbers of decoder layers.}
	\label{fig:decoder_layers}
\end{figure}

\subsection{Different Backbones.} We assess our model's performance with various pre-trained backbones, including a CNN-based backbone (ResNet-50) and two distinct pre-trained transformer backbones, namely Dino~\cite{caron2021emerging, oquab2023dinov2} and Swin V2~\cite{liu2022swin}.
Dino and DinoV2 are self-supervised Vision Transformers trained via self-distillation, resulting in robust, finely detailed semantic features. Moreover, these encoded semantic representations are shared among related but distinct object categories.
Swin Transformer restructures self-attention with a window mechanism, balancing efficiency and performance for vision tasks. This hierarchical architecture has the flexibility to model at different scales and has linear computational complexity with respect to image size.
As shown in Table~\ref{Tab:backbone}, SwinV2 outperforms other options, delivering superior results while maintaining efficiency comparable to the CNN-based backbone. In addition, using a larger backbone boosts performance, but at the price of efficiency and size.
\begin{table}
\centering
\caption{
\textbf{Pre-Trained Backbone Ablation.} PCK scores using different pre-trained backbones. Swin transformer combines superior results with efficient processing.
}
\small

\begin{tabular}{c|ccc}

\toprule
Backbone & \# Params[M] & FLOPS[G] & PCK$_{0.2}$ \\
\midrule
ResNet-50~\cite{he2016deep} & 25.5 & 4.1 & 87.71 \\
DinoV1-S~\cite{caron2021emerging} & 22.1 & 46.7 & 89.17 \\
DinoV2-S~\cite{oquab2023dinov2} & 22.1 & 46.7 &  90.34 \\
SwinV2-T~\cite{liu2022swin} & 28.3 & 4.4 & 91.19\\
SwinV2-S~\cite{liu2022swin} & 49.73 & 8.57 & 94.73\\

\bottomrule
\end{tabular}
\label{Tab:backbone}
\end{table}
