# Supplementary material for: A Graph-Based Approach for Category-Agnostic Pose Estimation
Source: arXiv:2311.17891 source file (2024-07-11)
Supplement: Supplementary file 2 [file 3_vis.tex]

\section{Qualitative Results}\label{supp_results}
\subsection{Further Results}
More qualitative results of POMNet~\cite{xu2022pose}, Capeformer~\cite{Shi_2023_CVPR}, Capeformer-T, and GraphCape are shown in Figures~\ref{fig:supp_qualitative} and~\ref{fig:supp_qualitative2}. Visualization of POMNet~\cite{xu2022pose} was done by training a network using the official code~\footnote{https://github.com/luminxu/Pose-for-Everything}, while for CapeFormer we used their publicly available code and pre-trained networks~\footnote{https://github.com/flyinglynx/CapeFormer/}.
\input{supp_figs/qualitative/qualitative}
\input{supp_figs/qualitative/qualitative2}

Furthermore, Figure~\ref{fig:sup_ood} shows additional out-of-distribution examples using our method.
\input{supp_figs/OOD/ood}
\subsection{Different Graph Definitions}
We also show in Figure~\ref{fig:sym_a} symmetry-breaking and structure-preserving examples, using partial keypoint definitions. In addition, we show qualitative results in Figure~\ref{fig:sym_b} using wrong skeleton inputs, validating the contribution of the graph decoder and the use of structural knowledge.
\input{supp_figs/symmetry/sym}

In addition, we experiment with different skeleton annotations for the same support image. As shown in the main paper, different graph definitions result in different performance. Qualitative results are shown in Figure~\ref{fig:skel}. Connecting symmetric nodes to unique nodes raises performance. We defer the exploration of determining the optimal skeletal relation to future research.
\input{supp_figs/skeleton/skeleton}

\subsection{Masking Experiments}
Additional qualitative results from the masking experiment, outlined in the main paper, are presented in Figures~\ref{fig:supp_mask_query} and~\ref{fig:supp_mask_supp}. 
Notably, in the last row of Figures~\ref{fig:supp_mask_query} and~\ref{fig:supp_mask_supp}, the structural prior proves beneficial for the model in localization, maintaining consistency in structure even under extreme masking conditions. This shows that our method is superior under masks and occlusions, which has many real-world implications.
In addition, the results indicate a significant performance decline when the query image is masked, contrasting with our model's robustness to significant masking of the support image. 
\begin{figure*}
\setlength{\fboxsep}{0pt}
\setlength{\fboxrule}{1.5pt}
  \centering
  \begin{tabular}{c ccc}
     Support & GT & CapeFormer-T & \textbf{GraphCape} \\

    \fcolorbox{purple}{white}{\includegraphics[width=0.2\textwidth]{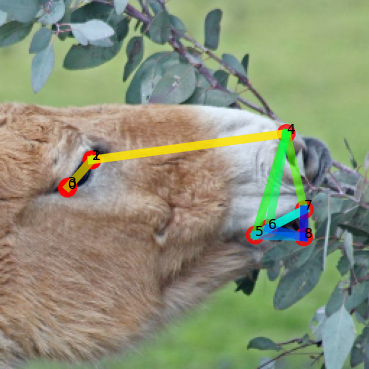}} & 
    \fcolorbox{ForestGreen}{white}{\includegraphics[width=0.2\textwidth]{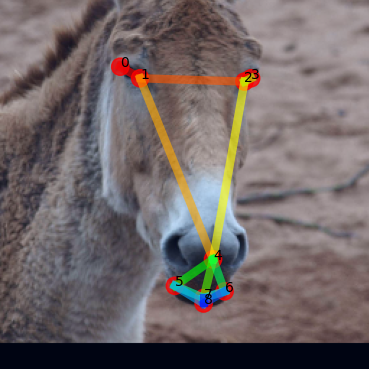}} & 
    \fcolorbox{ForestGreen}{white}{\includegraphics[width=0.2\textwidth]{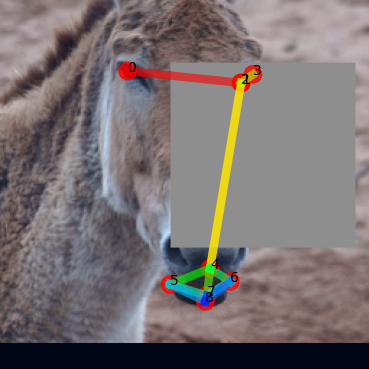}} &
    \fcolorbox{ForestGreen}{white}{\includegraphics[width=0.2\textwidth]{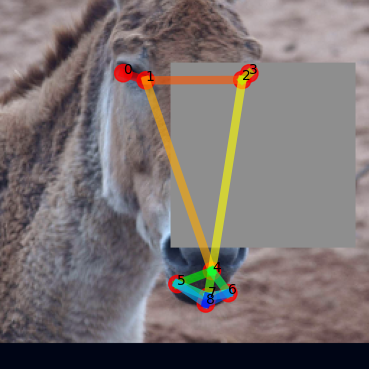}} \\

    \fcolorbox{purple}{white}{\includegraphics[width=0.2\textwidth]{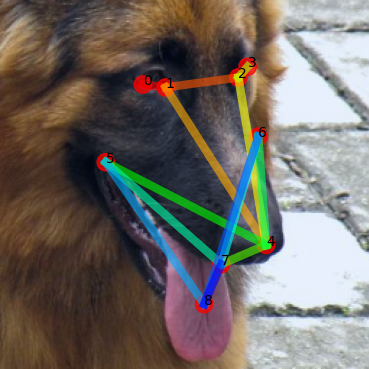}} & 
    \fcolorbox{ForestGreen}{white}{\includegraphics[width=0.2\textwidth]{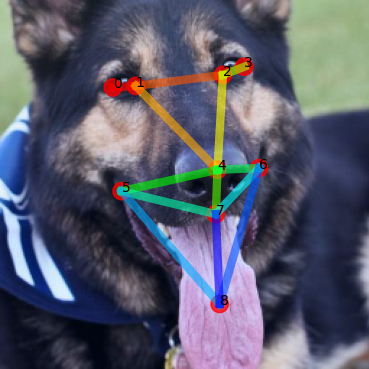}} & 
    \fcolorbox{ForestGreen}{white}{\includegraphics[width=0.2\textwidth]{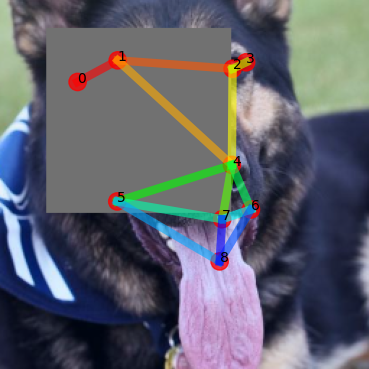}} &
    \fcolorbox{ForestGreen}{white}{\includegraphics[width=0.2\textwidth]{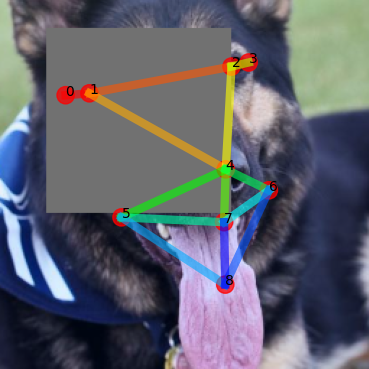}} \\

    %     \fcolorbox{purple}{white}{\includegraphics[width=0.2\textwidth]{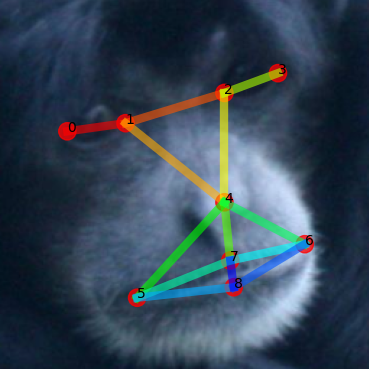}} & 
    % \fcolorbox{ForestGreen}{white}{\includegraphics[width=0.2\textwidth]{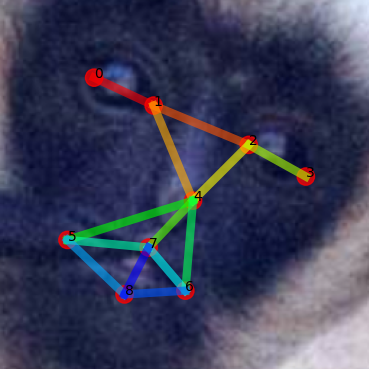}} & 
    % \fcolorbox{ForestGreen}{white}{\includegraphics[width=0.2\textwidth]{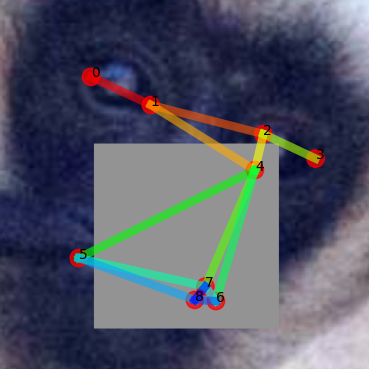}} &
    % \fcolorbox{ForestGreen}{white}{\includegraphics[width=0.2\textwidth]{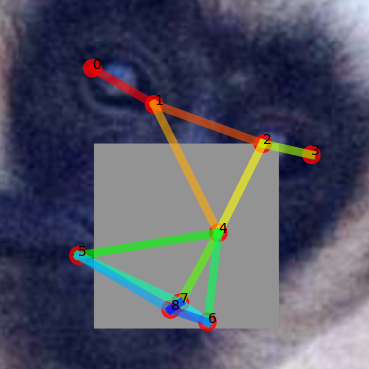}} \\

        \fcolorbox{purple}{white}{\includegraphics[width=0.2\textwidth]{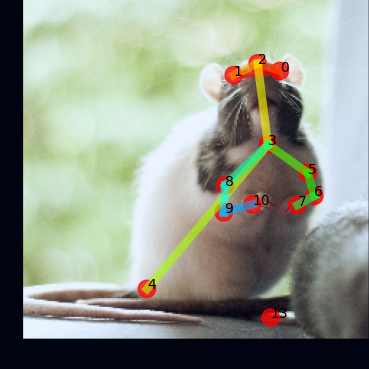}} & 
    \fcolorbox{ForestGreen}{white}{\includegraphics[width=0.2\textwidth]{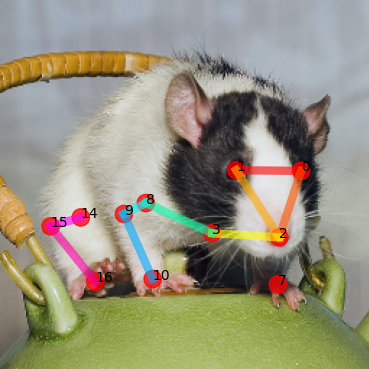}} & 
    \fcolorbox{ForestGreen}{white}{\includegraphics[width=0.2\textwidth]{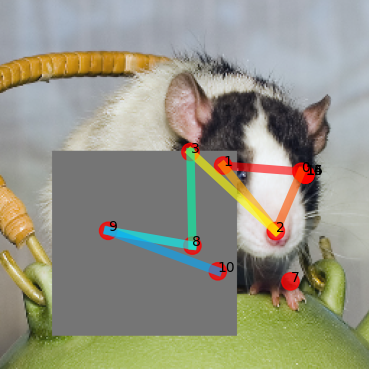}} &
    \fcolorbox{ForestGreen}{white}{\includegraphics[width=0.2\textwidth]{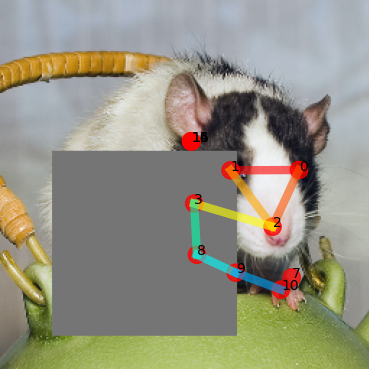}} \\

            \fcolorbox{purple}{white}{\includegraphics[width=0.2\textwidth]{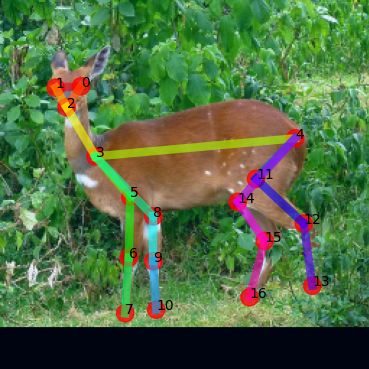}} & 
    \fcolorbox{ForestGreen}{white}{\includegraphics[width=0.2\textwidth]{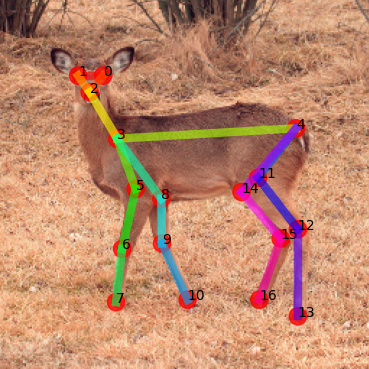}} & 
    \fcolorbox{ForestGreen}{white}{\includegraphics[width=0.2\textwidth]{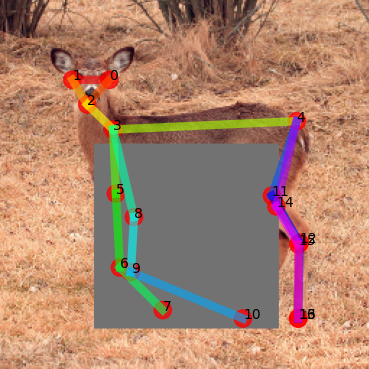}} &
    \fcolorbox{ForestGreen}{white}{\includegraphics[width=0.2\textwidth]{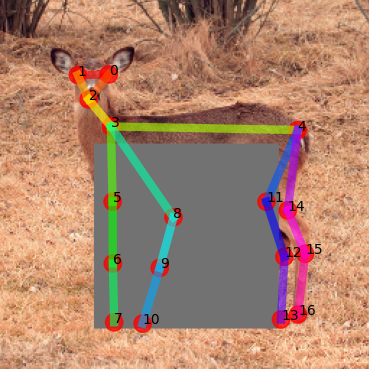}} \\
    
    %     \fcolorbox{purple}{white}{\includegraphics[width=0.2\textwidth]{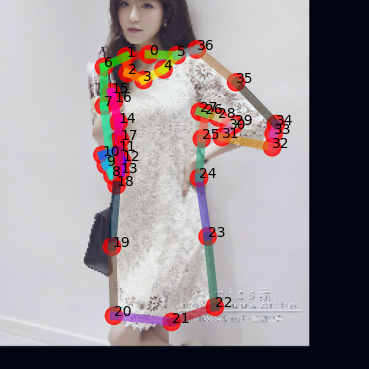}} & 
    % \fcolorbox{ForestGreen}{white}{\includegraphics[width=0.2\textwidth]{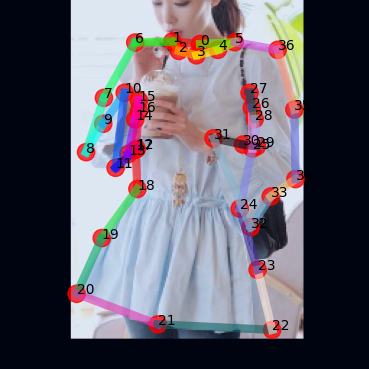}} & 
    % \fcolorbox{ForestGreen}{white}{\includegraphics[width=0.2\textwidth]{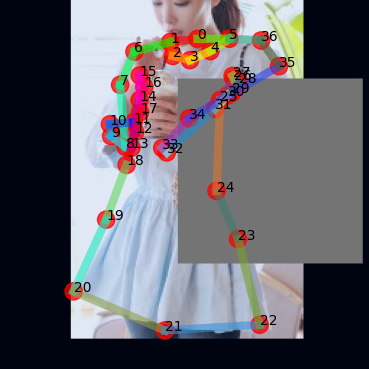}} &
    % \fcolorbox{ForestGreen}{white}{\includegraphics[width=0.2\textwidth]{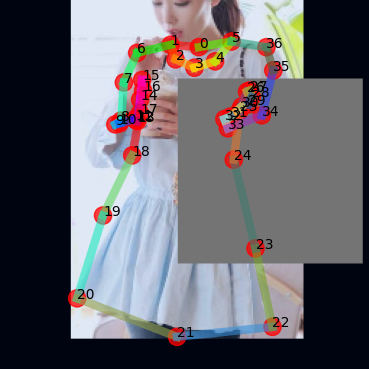}} \\

    %     \fcolorbox{purple}{white}{\includegraphics[width=0.2\textwidth]{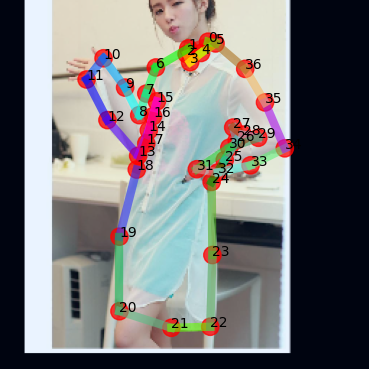}} & 
    % \fcolorbox{ForestGreen}{white}{\includegraphics[width=0.2\textwidth]{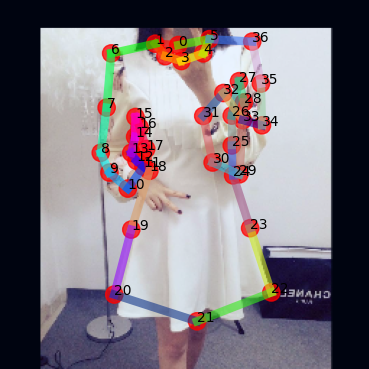}} & 
    % \fcolorbox{ForestGreen}{white}{\includegraphics[width=0.2\textwidth]{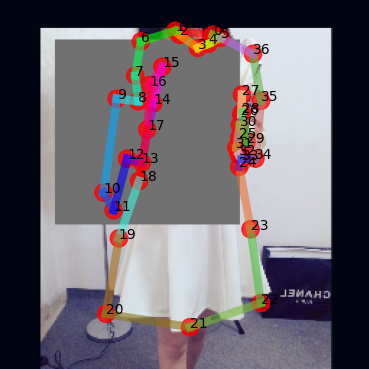}} &
    % \fcolorbox{ForestGreen}{white}{\includegraphics[width=0.2\textwidth]{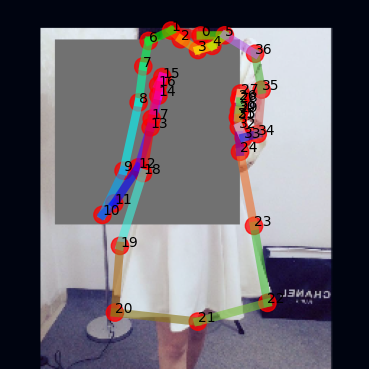}} \\

    \fcolorbox{purple}{white}{\includegraphics[width=0.2\textwidth]{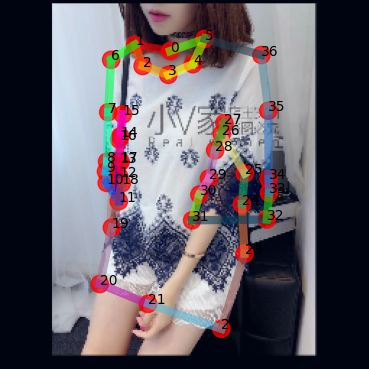}} & 
    \fcolorbox{ForestGreen}{white}{\includegraphics[width=0.2\textwidth]{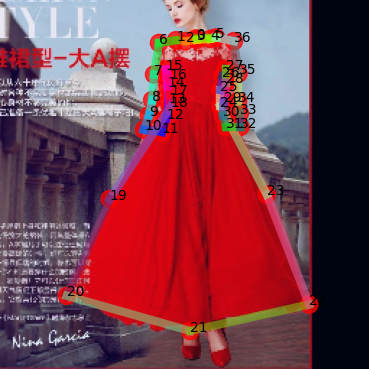}} & 
    \fcolorbox{ForestGreen}{white}{\includegraphics[width=0.2\textwidth]{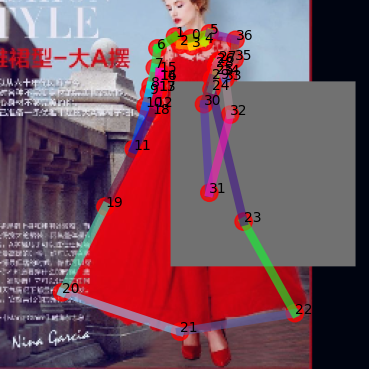}} &
    \fcolorbox{ForestGreen}{white}{\includegraphics[width=0.2\textwidth]{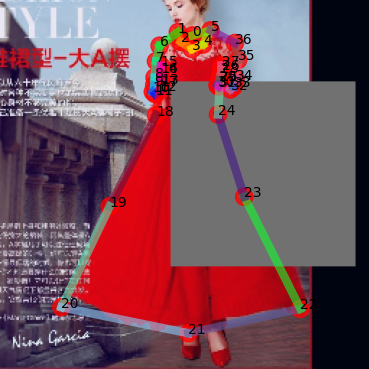}} \\

    \end{tabular}
  \caption{\textbf{Mask Query Results.} Qualitative results when masking the query image using the
enhanced baseline and our graph-based model. Although masking a large portion of the query image, using structure bias helps preserve structure consistency and break symmetry.
  }
  \label{fig:supp_mask_query}
\end{figure*}

\begin{figure*}
\setlength{\fboxsep}{0pt}
\setlength{\fboxrule}{1.5pt}
  \centering
  \begin{tabular}{c ccc}
     Support & GT & CapeFormer-T & \textbf{GraphCape} \\

    \fcolorbox{purple}{white}{\includegraphics[width=0.2\textwidth]{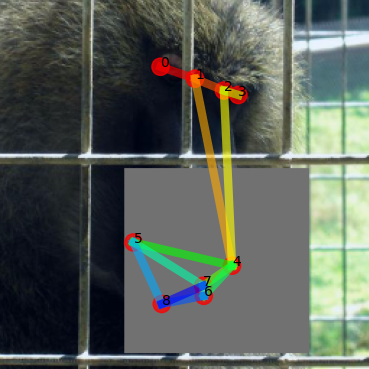}} & 
    \fcolorbox{ForestGreen}{white}{\includegraphics[width=0.2\textwidth]{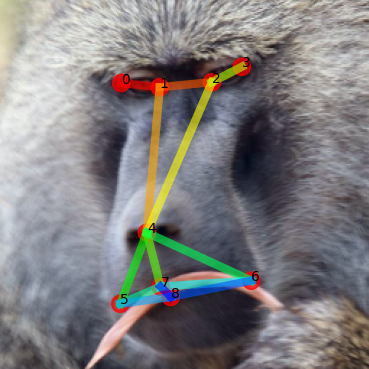}} & 
    \fcolorbox{ForestGreen}{white}{\includegraphics[width=0.2\textwidth]{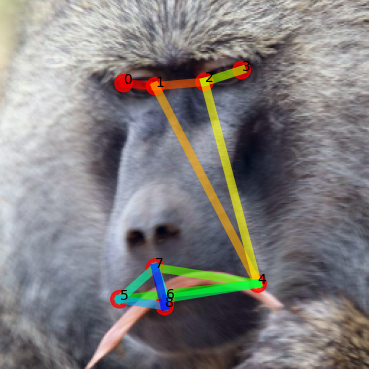}} &
    \fcolorbox{ForestGreen}{white}{\includegraphics[width=0.2\textwidth]{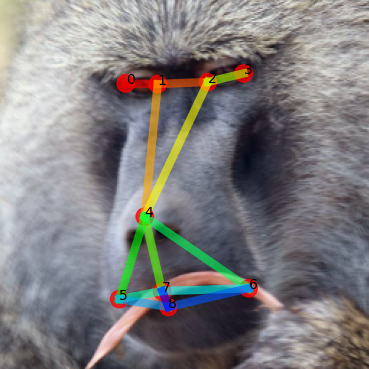}} \\

    \fcolorbox{purple}{white}{\includegraphics[width=0.2\textwidth]{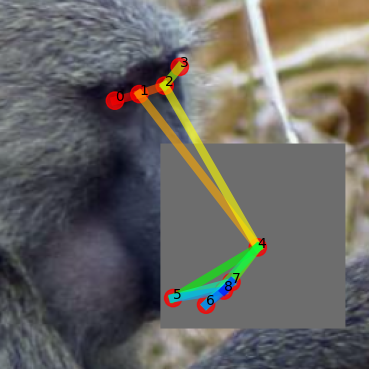}} & 
    \fcolorbox{ForestGreen}{white}{\includegraphics[width=0.2\textwidth]{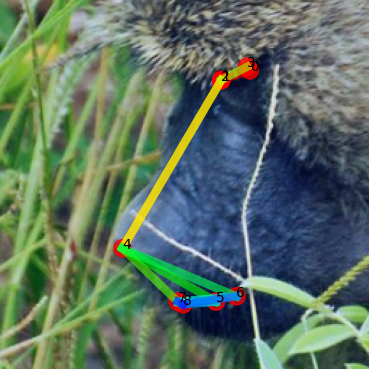}} & 
    \fcolorbox{ForestGreen}{white}{\includegraphics[width=0.2\textwidth]{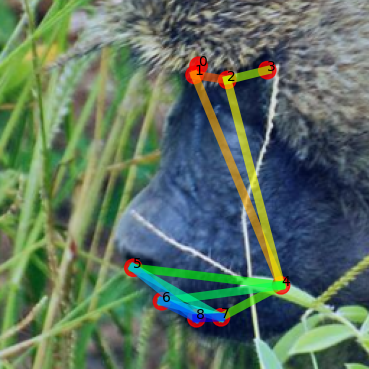}} &
    \fcolorbox{ForestGreen}{white}{\includegraphics[width=0.2\textwidth]{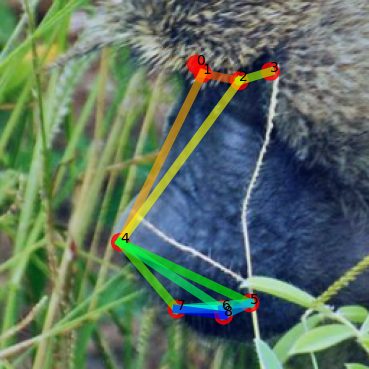}} \\

    \fcolorbox{purple}{white}{\includegraphics[width=0.2\textwidth]{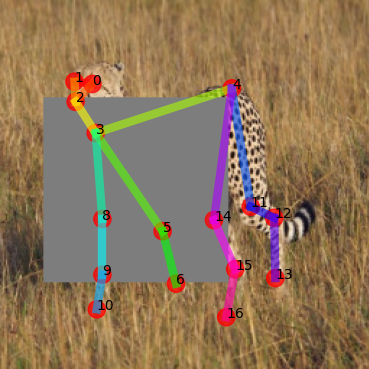}} & 
    \fcolorbox{ForestGreen}{white}{\includegraphics[width=0.2\textwidth]{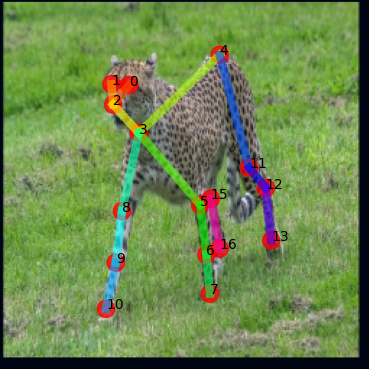}} & 
    \fcolorbox{ForestGreen}{white}{\includegraphics[width=0.2\textwidth]{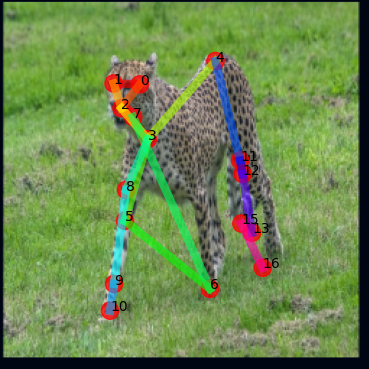}} &
    \fcolorbox{ForestGreen}{white}{\includegraphics[width=0.2\textwidth]{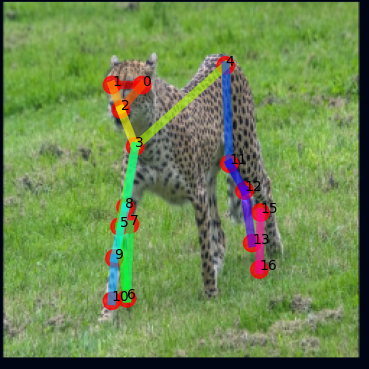}} \\

    \fcolorbox{purple}{white}{\includegraphics[width=0.2\textwidth]{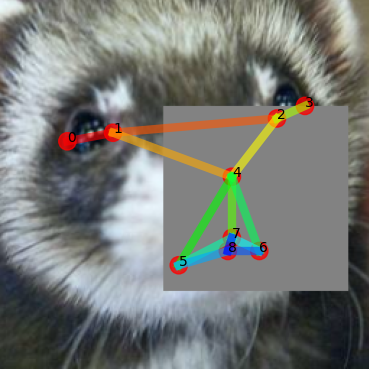}} & 
    \fcolorbox{ForestGreen}{white}{\includegraphics[width=0.2\textwidth]{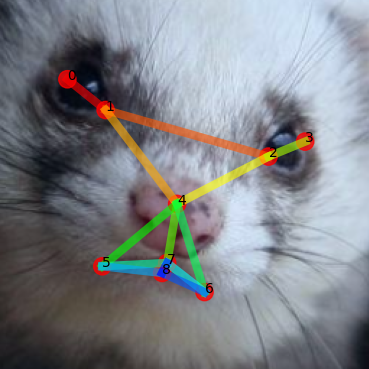}} & 
    \fcolorbox{ForestGreen}{white}{\includegraphics[width=0.2\textwidth]{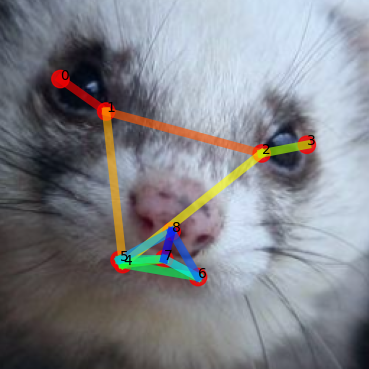}} &
    \fcolorbox{ForestGreen}{white}{\includegraphics[width=0.2\textwidth]{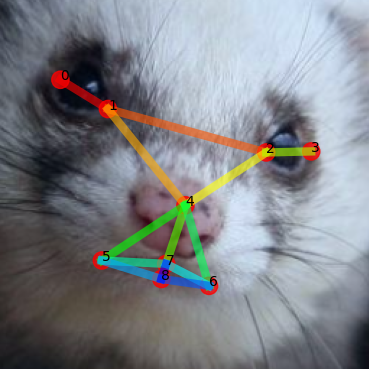}} \\

    \fcolorbox{purple}{white}{\includegraphics[width=0.2\textwidth]{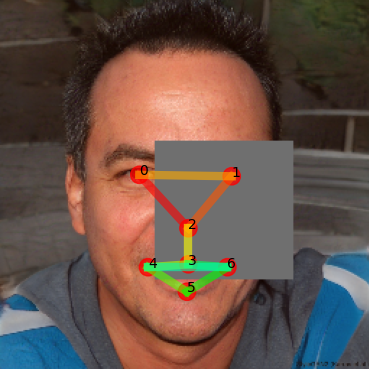}} &
    \fcolorbox{ForestGreen}{white}{\includegraphics[width=0.2\textwidth]{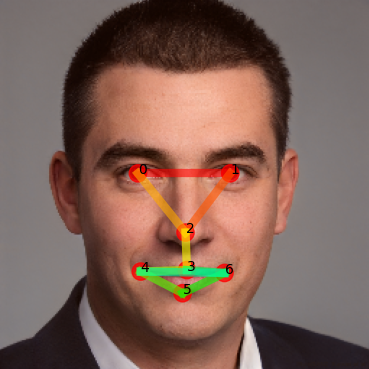}} &
    \fcolorbox{ForestGreen}{white}{\includegraphics[width=0.2\textwidth]{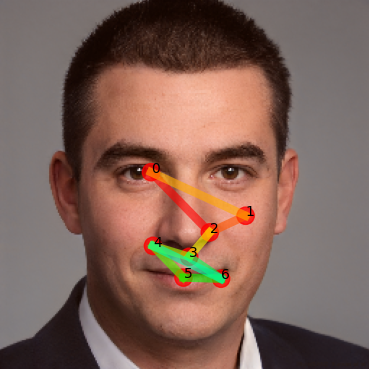}} &
    \fcolorbox{ForestGreen}{white}{\includegraphics[width=0.2\textwidth]{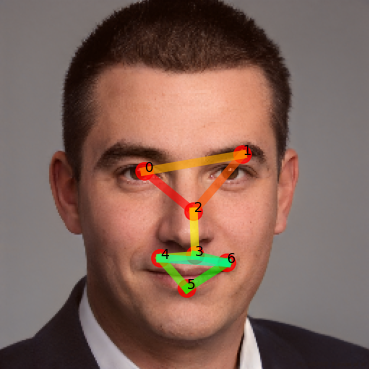}} \\
    
    % \fcolorbox{purple}{white}{\includegraphics[width=0.2\textwidth]{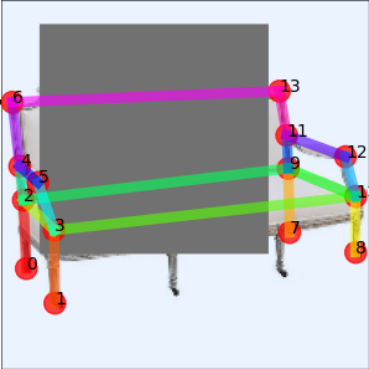}} & 
    % \fcolorbox{ForestGreen}{white}{\includegraphics[width=0.2\textwidth]{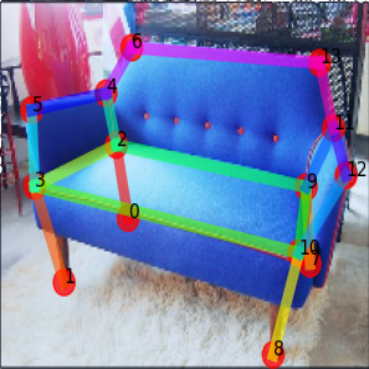}} & 
    % \fcolorbox{ForestGreen}{white}{\includegraphics[width=0.2\textwidth]{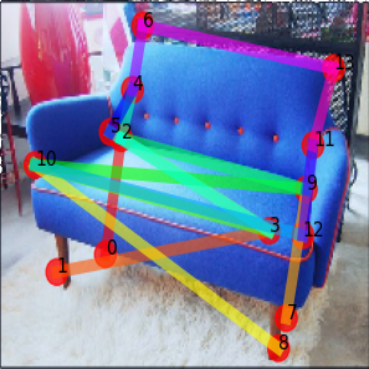}} &
    % \fcolorbox{ForestGreen}{white}{\includegraphics[width=0.2\textwidth]{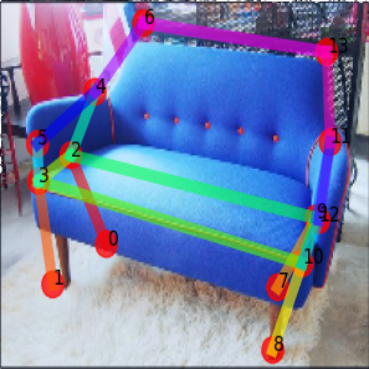}} \\
    \end{tabular}
  \caption{\textbf{Mask Support Results.} Qualitative results when masking the support image using the
enhanced baseline and our graph-based model. Our model can predict keypoints even when a significant portion of the support image is masked, leveraging the power of graph structure.
  }
  \label{fig:supp_mask_supp}
\end{figure*}
