# Supplementary material for: A Graph-Based Approach for Category-Agnostic Pose Estimation
Source: arXiv:2311.17891 source file (2024-07-11)
Supplement: Supplementary file 4 [file 1_intro.tex]

\input{supp_figs/teaser/teaser}
The following sections include additional information about our method. 

Section~\ref{supp:details} offers additional details about our method, explores alternative architectural decisions, and provides a brief overview of our endeavor to integrate structure as a loss term. 
Section~\ref{supp_exp} presents the experimental findings on the scalability of our design and further ablation studies. 
Lastly, Section~\ref{supp_results} showcases qualitative comparisons of our method on the MP-100 dataset, further results of our masking experiment, and examples illustrating symmetry cases and outcomes using various skeleton annotations.
