# Supplementary material for: A Graph-Based Approach for Category-Agnostic Pose Estimation
Source: arXiv:2311.17891 source file (2024-07-11)
Supplement: Supplementary file 5 [file query_mask.tex]

\begin{figure*}
\setlength{\fboxsep}{0pt}
\setlength{\fboxrule}{1.5pt}
  \centering
  \begin{tabular}{c ccc}
     Support & GT & CapeFormer-T & \textbf{GraphCape} \\

    \fcolorbox{purple}{white}{\includegraphics[width=0.2\textwidth]{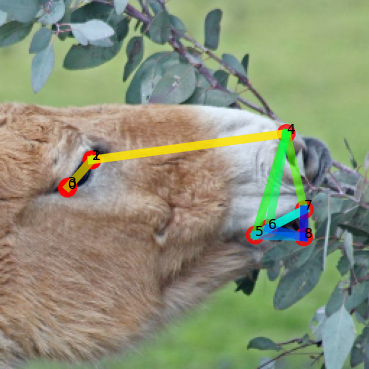}} & 
    \fcolorbox{ForestGreen}{white}{\includegraphics[width=0.2\textwidth]{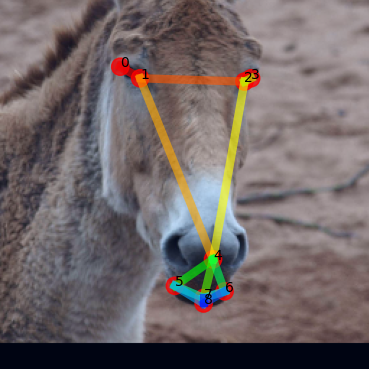}} & 
    \fcolorbox{ForestGreen}{white}{\includegraphics[width=0.2\textwidth]{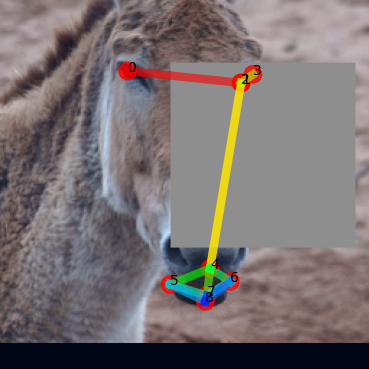}} &
    \fcolorbox{ForestGreen}{white}{\includegraphics[width=0.2\textwidth]{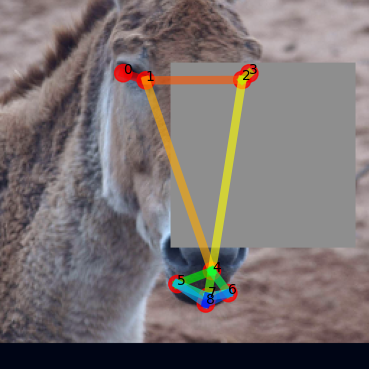}} \\

    \fcolorbox{purple}{white}{\includegraphics[width=0.2\textwidth]{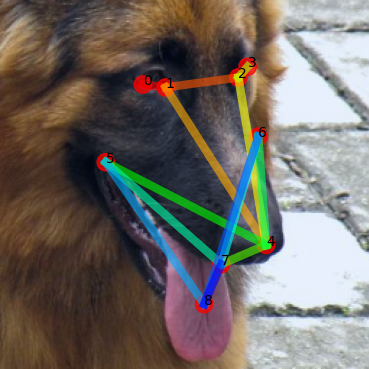}} & 
    \fcolorbox{ForestGreen}{white}{\includegraphics[width=0.2\textwidth]{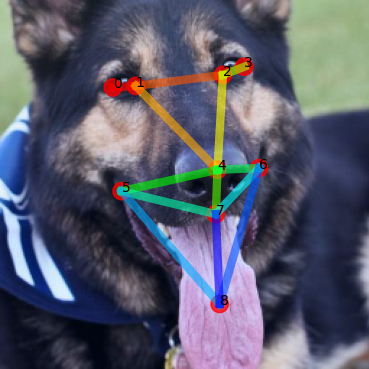}} & 
    \fcolorbox{ForestGreen}{white}{\includegraphics[width=0.2\textwidth]{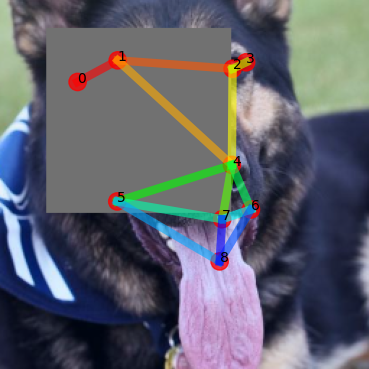}} &
    \fcolorbox{ForestGreen}{white}{\includegraphics[width=0.2\textwidth]{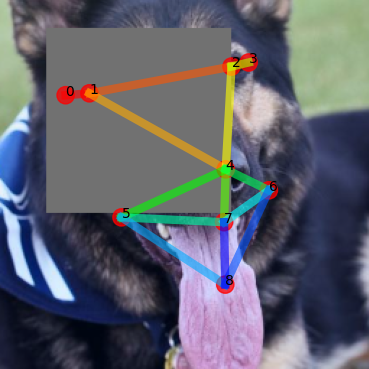}} \\

    %     \fcolorbox{purple}{white}{\includegraphics[width=0.2\textwidth]{supp_figs/mask/query/38_0.png}} & 
    % \fcolorbox{ForestGreen}{white}{\includegraphics[width=0.2\textwidth]{supp_figs/mask/query/gt_38_1.png}} & 
    % \fcolorbox{ForestGreen}{white}{\includegraphics[width=0.2\textwidth]{supp_figs/mask/query/base_38_1.png}} &
    % \fcolorbox{ForestGreen}{white}{\includegraphics[width=0.2\textwidth]{supp_figs/mask/query/38_1.png}} \\

        \fcolorbox{purple}{white}{\includegraphics[width=0.2\textwidth]{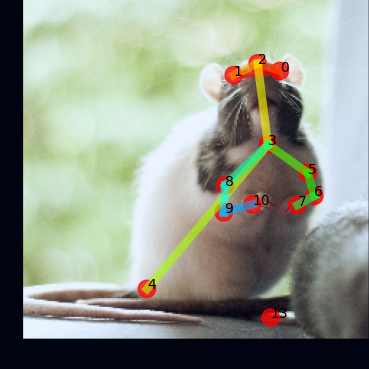}} & 
    \fcolorbox{ForestGreen}{white}{\includegraphics[width=0.2\textwidth]{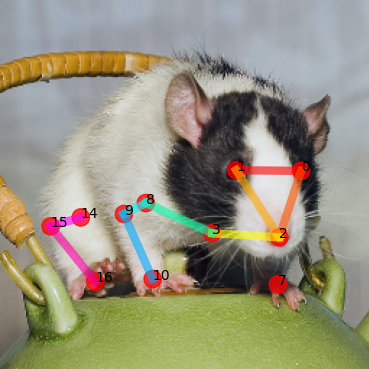}} & 
    \fcolorbox{ForestGreen}{white}{\includegraphics[width=0.2\textwidth]{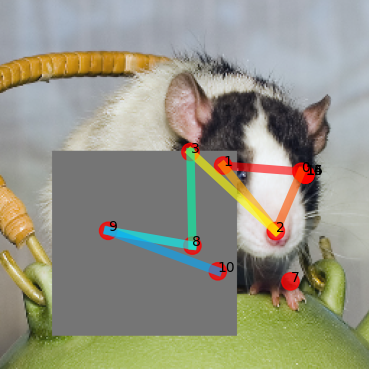}} &
    \fcolorbox{ForestGreen}{white}{\includegraphics[width=0.2\textwidth]{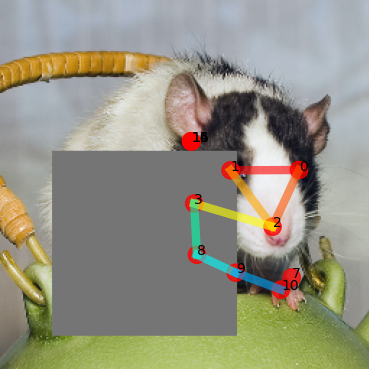}} \\

            \fcolorbox{purple}{white}{\includegraphics[width=0.2\textwidth]{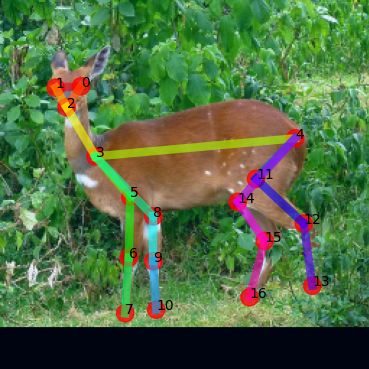}} & 
    \fcolorbox{ForestGreen}{white}{\includegraphics[width=0.2\textwidth]{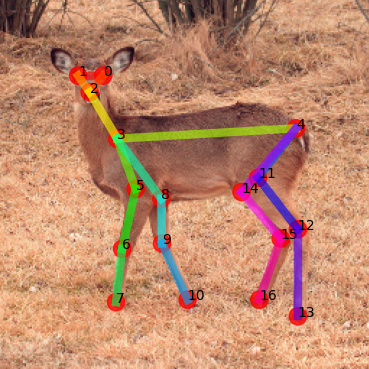}} & 
    \fcolorbox{ForestGreen}{white}{\includegraphics[width=0.2\textwidth]{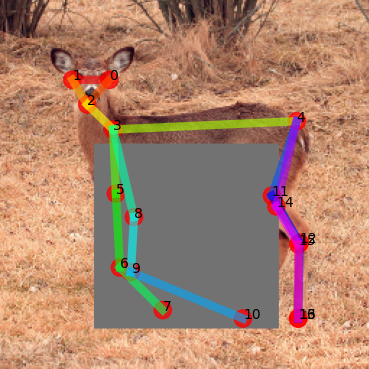}} &
    \fcolorbox{ForestGreen}{white}{\includegraphics[width=0.2\textwidth]{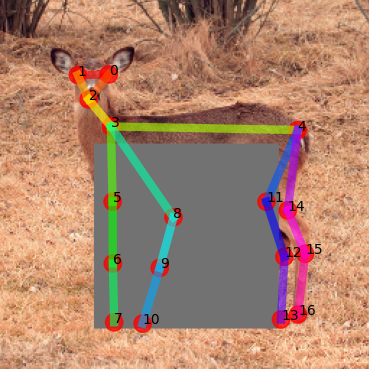}} \\
    
    %     \fcolorbox{purple}{white}{\includegraphics[width=0.2\textwidth]{supp_figs/mask/query/78_0.png}} & 
    % \fcolorbox{ForestGreen}{white}{\includegraphics[width=0.2\textwidth]{supp_figs/mask/query/gt_78_1.png}} & 
    % \fcolorbox{ForestGreen}{white}{\includegraphics[width=0.2\textwidth]{supp_figs/mask/query/base_78_1.png}} &
    % \fcolorbox{ForestGreen}{white}{\includegraphics[width=0.2\textwidth]{supp_figs/mask/query/78_1.png}} \\

    %     \fcolorbox{purple}{white}{\includegraphics[width=0.2\textwidth]{supp_figs/mask/query/79_0.png}} & 
    % \fcolorbox{ForestGreen}{white}{\includegraphics[width=0.2\textwidth]{supp_figs/mask/query/gt_79_1.png}} & 
    % \fcolorbox{ForestGreen}{white}{\includegraphics[width=0.2\textwidth]{supp_figs/mask/query/base_79_1.png}} &
    % \fcolorbox{ForestGreen}{white}{\includegraphics[width=0.2\textwidth]{supp_figs/mask/query/79_1.png}} \\

    \fcolorbox{purple}{white}{\includegraphics[width=0.2\textwidth]{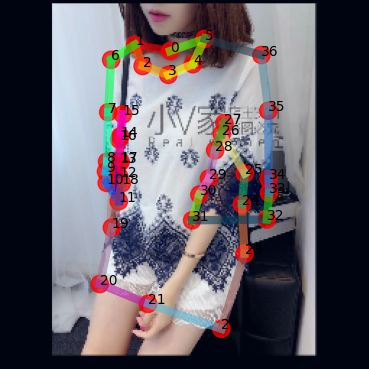}} & 
    \fcolorbox{ForestGreen}{white}{\includegraphics[width=0.2\textwidth]{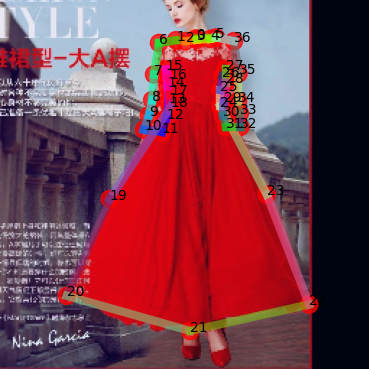}} & 
    \fcolorbox{ForestGreen}{white}{\includegraphics[width=0.2\textwidth]{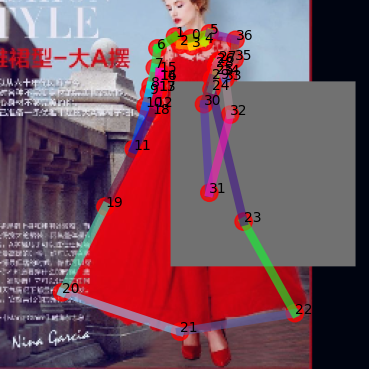}} &
    \fcolorbox{ForestGreen}{white}{\includegraphics[width=0.2\textwidth]{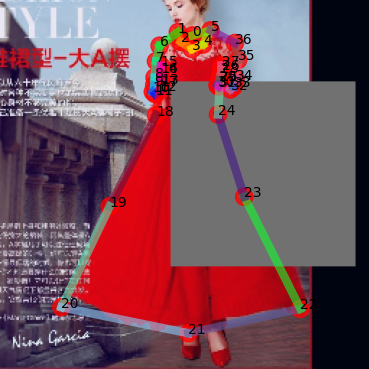}} \\

    \end{tabular}
  \caption{\textbf{Mask Query Results.} Qualitative results when masking the query image using the
enhanced baseline and our graph-based model. Although masking a large portion of the query image, using structure bias helps preserve structure consistency and break symmetry.
  }
  \label{fig:supp_mask_query}
\end{figure*}
